# Supplementary material for: Magnetoresistance in ZrSi$X$ ($X=$ S, Se, Te) nodal-line semimetals
Source: arXiv:2504.12547 ancillary file (2025-04-17)
Supplement: Supplementary file 1 [file SM.pdf]

# Supplemental Material for
# "Magnetoresistance in ZrSi$X$ ($X$ = S, Se, Te) nodal-line semimetals"

ShengNan Zhang[1,2,3,*] and Oleg V. Yazyev[1,2,†]

[1] *Institute of Physics, Ecole Polytechnique Fédérale de Lausanne (EPFL), CH-1015 Lausanne, Switzerland*
[2] *National Centre for Computational Design and Discovery of Novel Materials MARVEL, Ecole Polytechnique Fédérale de Lausanne (EPFL), CH-1015 Lausanne, Switzerland*
[3] *Beijing Polytechnic College, Beijing 100042, China*

### A. Magnetoresistance and Fermi surface of ZrSiSe

We commence our discussion by presenting the calculated magnetoresistance (MR) of ZrSiSe in Fig. S1. Given the very similar crystal structures of ZrSiS and ZrSiSe [1], their diamond-shaped Fermi surfaces appear strikingly similar too (Fig. S2). However, there exist subtle yet noteworthy differences. For the electron pocket, there is no significant difference from the side view. However, four separate pieces in the Fermi surface of ZrSiS consolidate into a single, continuous entity in the Fermi surface of ZrSiSe when observed from the top view. Additionally, the tube-shaped hole pockets in ZrSiS transform into closed structures in ZrSiSe, implying the absence of open orbits in the magnetotransport and, hence, leading to distinct variations in the MR results. It is important to note that the Fermi surface depicted in Fig. S2 represents only a fraction of the quasi-particles participating in the transport. Those in close proximity to the Fermi energy also deserve consideration. Figs. S2(c) and S2(d) illustrate the isoenergy surface for $E = E_{\mathrm{F}} - 0.01$ eV. While the electron pocket does not exhibit significant alteration, the initially disconnected hole pockets transform into tube-shaped structures extending along the $c$ axis. Overall, the entire Fermi surface maintains structural similarity to that of ZrSiS, explaining why their MR properties show resemblance.

As a result, the anisotropic magnetoresistance (MR) of ZrSiSe bears a close resemblance to that of ZrSiS. We depict the anisotropic MR in Figs. S1(a) and S1(b), when the magnetic field is rotated in the $a$-$c$ plane and the $a$-$b$ plane, respectively. The calculated MR corresponds well to the experimental measurements reported in Ref. [2]. Following the same analysis as for ZrSiS, the butterfly-shaped anisotropic MR of ZrSiSe (Fig. S1(a)) can be attributed to the intricate fine structure of its Fermi surface. This results in a complex mixture of electron and hole charge carriers trajectories, leading to a non-monotonic variation of MR. The anisotropic MR exhibits a four-fold symmetry (Fig. S1 (b)) when the magnetic field is rotated in the $a$-$b$ plane, owing to the $C_{4z}$ symmetry of the Fermi surface in the $a$-$b$ plane. For the magnetic field is oriented along the $a$ axis, the resistivity obtains its maximum due to the open orbits from the hole Fermi surface pocket.

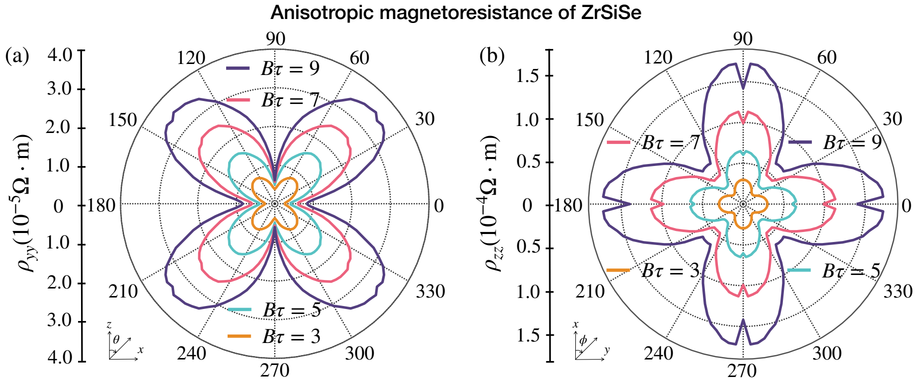


FIG. S1. Calculated anisotropic magnetoresistivity of ZrSiSe for current along (a) the $b$ and (b) $c$ axes, and magnetic field rotating in the $a$-$c$ and $a$-$b$ planes, respectively.

* shengnan.zhang@epfl.ch
† oleg.yazyev@epfl.ch

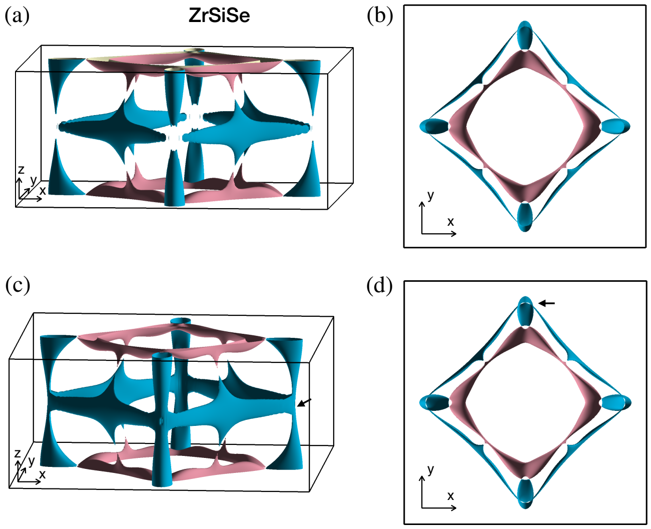


FIG. S2. (a) Side view and (b) top view of the Fermi surface of ZrSiSe show no open orbits along the $c$ axis. (c),(d) Same views of the isoenergy surface at $-0.01$ eV relative to the Fermi energy show the emergence of open-orbit segments marked by arrows.

[1] Q. Xu, Z. Song, S. Nie, H. Weng, Z. Fang, and X. Dai, Phys. Rev. B **92**, 205310 (2015).
[2] Y.-C. Chiu, K.-W. Chen, R. Schönemann, V. L. Quito, S. Sur, Q. Zhou, D. Graf, E. Kampert, T. Förster, K. Yang, G. T. McCandless, J. Y. Chan, R. E. Baumbach, M. D. Johannes, and L. Balicas, Phys. Rev. B **100**, 125112 (2019).
